# Supplementary material for: When random walkers help solving intriguing integrals
Source: arXiv:1906.04545 ancillary file (2019-06-11)
Supplement: Supplementary file 1 [file supp_mat5.pdf]

# When random walkers help solving intriguing integrals: supplemental material

Satya N. Majumdar and Emmanuel Trizac
*LPTMS, CNRS, Univ. Paris-Sud, Université Paris-Saclay, 91405 Orsay, France*
(Dated: June 11, 2019)

We give here the principal arguments or details behind the calculations described in the manuscript. We start in section I by showing how to treat the $J_N$ integrals along similar lines as those invoked for their $I_N$ counterpart. The idea is summarized in I A; it relies on a symmetry property that is worked out in I B. As a side comment, an alternative route to identity (7) is presented in I C. We then prove Eqs. (15) and (16) of the main text in section II. Section III is devoted to revisiting our causality argument, in a situation where a spreading packet of walkers on a line undergo a left-right symmetric random walk; the packet will exhibit a fixed center-of-mass, until the front of the packet hits a boundary, which impinges on symmetry. This is associated to a change of behavior for a new class of integrals. This situation is the reverse of that discussed in the main paper, where a "message" was traveling from the edge of the system, to its center. Here, the messengers will start from the center and travel towards the edges. Finally, we show in section IV that it is sufficient to work with functions that have a bounded Fourier transform.

## I. THE RANDOM WALK REFORMULATION FOR THE $J_N$-TYPE INTEGRALS

### A. Summarizing the argument

In order to treat integrals $J_N$ defined in Eq. (2) of the main text, we invoke (5)

$$p_N(a_1) = \int \frac{dk}{2\pi} \cos(ka_1) \prod_{n=1}^{N} \text{sinc}(a_n k). \tag{S1}$$

Thus, we evaluate the same object as before $p_N(x)$, at $x = a_1$, at the boundary of the domain spanned by the first step. The left/right symmetry of the steps $n = 2$, $n = 3$ etc. preserves the "edge" density $p_N(a_1)$, which has to be exactly half of $p_1(0) = 1/(2a_1)$. This property will be derived in the next subsection; it is visible in Fig. 1 of the main text, and holds until the "messengers", now originating from the second edge at $x = -a_1$, do reach $x = a_1$. They have to travel a distance $2a_1$, twice larger than previously, see below. This tells us that $J_1 = J_2 = \ldots = \pi/2$, under the proviso that $\sum_{n=2}^{N} a_n < 2\,a_1$, and we recover the exact result established in [1, 2]. This constraint is looser than that applying to $I_N$ integrals (i.e. $\sum_{n=2}^{N} a_n < a_1$), since the messengers now have to travel twice a larger distance.

### B. Symmetry argument for the "edge" density

The $J_N$ type of integrals, from Eq. (S1) above, are related to the density of walkers at $x = a_1$, at the edge of the domain spanned by the first jump of the random walk ($[-a_1, a_1]$). Unlike the walkers that are located close to $x = 0$, those at $x = a_1$ do know they sit at an edge, therefore in a non-infinite world. Yet, a simple symmetry argument shows that unless the walkers having started their journey from the other edge after the first jump (i.e. at $x = -a_1$), have reached $x = a_1$, then $p_N(a_1) = p_N(0)/2$. It turns convenient to this end to introduce a fictitious density of walkers, denoted $\mathcal{P}$ for "phantom", such that after step 1, the regular walkers are uniform in $[-a_1, a_1]$ while the $\mathcal{P}$ walkers are uniform in $[a_1, 3a_1]$, with the same density. $\mathcal{P}$ walkers are non interacting, do not interact with regular ones, but all follow the same random walk. Considering the total (regular + phantom) density of walkers, $p_N^{total}$, we are back to the problem treated in the main text, but for the fact that we have a twice more extended system after step 1, spanning an interval of length $4a_1$ rather than $2a_1$ (see Fig. S1 where $a_1 = 1$). Consequently, $p_N^{total}(a_1) = 1/(2a_1)$, under the proviso that $\sum_{n=2}^{N} a_n < 2a_1$. To connect $p_N^{total}(a_1)$ to $p_N(a_1)$, which is the desired quantity, we invoke the left-right symmetry of each step of the random walk. It implies first that the left and right tails of the regular walker density are symmetric with respect to $x = 0$, and that that the right tail of the regular walkers density $p_N$ and the left tail of the phantom walker density (denoted $p_N^{\mathcal{P}}$) are symmetric with respect to $x = a_1$ (see Fig. S1). More specifically, at $x = a_1$, we have $p_N(a_1) = p_N^{\mathcal{P}}(a_1)$, see the bullet in Fig S1-b. As a consequence, $p_N(a_1) = p_N^{total}(a_1)/2 = 1/(4a_1)$ for $\sum_{n=2}^{N} a_n < 2a_1$. This shows that $J_N = \pi/2$ for all $N$ and jump sizes fulfilling the constraint $\sum_{n=2}^{N} a_n < 2a_1$.

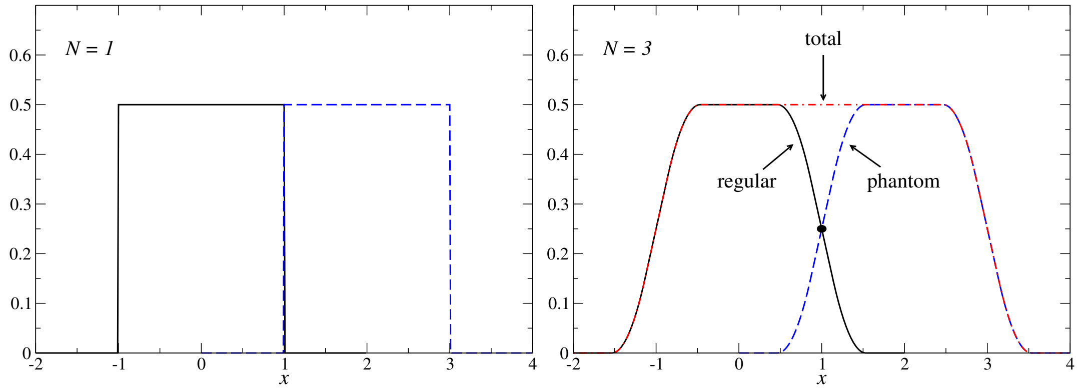


FIG. S1. (Color online) The phantom walkers arguments. The density of phantom walkers is shown with the dashed blue line while the continuous black curve is for the regular walkers. Left (a): After step 1 of the random walk, phantom walkers are introduced in the system, with a uniform density. Considering regular and phantom walkers altogether, we are back to the situation we started from in the main text, and a uniform density of walkers in $[-a_1, 3a_1]$ (here, $a_1 = 1$). Provided the walkers starting from the edges (regular walkers at $x = -a_1$ and phantom walkers at $x = 3a_1$) have not reached the center at $x = a_1$, we thus have $p_N^{total}(a_1) = p_1^{total}(a_1) = 1/(2a_1)$. Indeed, the total density of walkers (red dash-dotted line) is uniform near $x = a_1$. Such a situation, meaning $\sum_{n=2}^N a_n < 2a_1$ which we assume throughout, is depicted in the right panel (b) where we show for concreteness the case $N = 3$, $a_1 = 1$, $a_2 = 1/3$ and $a_3 = 1/5$. Besides, the left/right symmetry of each random step leads to the symmetry in the density of regular and phantom walkers, with respect to $x = a_1$ (right panel). Regular and phantom walkers thus have the same density at $x = a_1$ (see the bullet), so that $p_N(a_1) = p_N^{tot}(a_1)/2 = 1/4$ on the Figure.

### C. Recovering identity (7)

We stress that Eq. (S1) can be invoked for an alternative route to Eq. (7), which reads

$$\int_{-\infty}^{\infty} \cos(a_1 k) \prod_{n=2}^{N} \mathrm{sinc}(a_n\, k)\, dk \;=\; 0. \tag{S2}$$

Indeed, starting from $x = 0$, we consider now $p_{N-1}(a_1)$ to evaluate the density at $x = a_1$ for a walk made up of steps $n = 2$, $n = 3$ etc. This series of steps is too localized when the condition $\sum_{n=2}^N a_n \;<\; a_1$ prevents the walkers to reach the point $x = a_1$: $p_{N-1}(a_1) = 0$ so that the integral vanishes in (S2). With the argument presented in the main text, the vanishing result in (S2) stems from the origin being void of walkers after $N$ steps.

## II. PROOF OF EQS. (15) AND (16) OF THE MAIN TEXT

We consider a 4-step random walk in $d = 2$. The walker starts at the origin $O : (0, 0)$ in the $2d$ plane. In step 1, it jumps $\pm 1$ (with equal probability) along the $x$ direction. In step 2, it again jumps $\pm 1$ (with equal probability), but now along the $y$-direction. For a particular configuration, see Fig. S2-a, where after step 2, the walker arrives at $O' : (1, 1)$. Following step 2, the walker makes an isotropic Pearson jump of fixed radius $b$, where the end point of this step (denoted by $B$ in Fig. S2-a) is chosen uniformly on the circle of radius $b$. Finally, at the 4-th step, the walker makes another isotropic Pearson jump of radius $a$, with the endpoint $A$ chosen uniformly on the circle of radius $a$ (see Fig. S2-a). Without loss of generality, we consider $a < b$. At the end of the 4-th step, the Fourier transform of the position distribution $\widetilde{p}_4(\boldsymbol{k})$ is given by the product of the characteristic functions of the 4 jumps, since they are independent. Hence one gets

$$\widetilde{p}_4(\boldsymbol{k}) = \cos(k_x)\, \cos(k_y)\, J_0(b\, k)\, J_0(a\, k) \tag{S3}$$

where $k = \sqrt{k_x^2 + k_y^2}$ and for the 3rd and the 4th steps, we have used the formula in line (ii) of Eq. (10) in the main text with $d = 2$ and $S_2 = 2\pi$. Consequently, the position pdf is given by the Fourier inversion,

$$p_4(\boldsymbol{r}) = \int_{-\infty}^{\infty} \frac{dk_x}{2\pi} \int_{-\infty}^{\infty} \frac{dk_y}{2\pi}\, \widetilde{p}_4(\boldsymbol{k})\, e^{-i\boldsymbol{k}\cdot\boldsymbol{r}}. \tag{S4}$$

In particular, the pdf at the origin, i.e, the probability (density) to come back to the origin after 4 steps, is given by the double integral

$$p_4(\mathbf{0}) = \int_{\mathbb{R}^2} \frac{dk_x}{2\pi}\,\frac{dk_y}{2\pi}\, \cos(k_x)\, \cos(k_y)\, J_0(b\,k)\, J_0(a\,k)\,. \tag{S5}$$

This yields the left hand side (lhs) of Eq. (15) of the main text (times a factor $1/4\pi^2$).

Now, let us compute $p_4(\mathbf{0})$ directly by an elementary method. To this end, we ask the following question: starting from a point $B$ chosen uniformly on the circle of radius $b$ (centered at $O' : (1, 1)$ in Fig. S2-a) (just before the 4-th step), if a walker makes an isotropic jump of radius $a < b$, what is the probability (density) $p_4(\mathbf{0})$ that it will end up at the origin $O : (0, 0)$? To make the computation simple, we make use of the circular symmetry and transform Fig. S2-a to Fig. S2-b. The point $O' : (1, 1)$ is at a distance $\sqrt{2}$ from the origin $O : (0, 0)$ in Fig. S2-a. Hence, we can construct a new figure (Fig. S2-b) with a circle of radius $b$ centered at $O'$, we call this a new origin $O' : (0, 0)$ in Fig. S2-b. The target point $O$ is just a distance $\sqrt{2}$ from this center $O'$, and without loss of generality, we can take this target point $O$ to be on the new $x$ axis in Fig. S2b, i.e., $O : (\sqrt{2}, 0)$. Now, we choose a point $B$ uniformly on the circle of radius $b$, say it has the co-ordinate $(b\cos\phi, b\sin\phi)$ where $\phi$ is the angle shown in Fig. S2-b. The probability distribution of $B$ is uniform on the circle. Now, starting from B, we make an isotropic jump of fixed length $a$, characterized by the pdf $q(\boldsymbol{r}) = \frac{1}{2\pi a}\,\delta(r-a)$, where $r = |\boldsymbol{r}|$ and evidently $q(\boldsymbol{r})$ is normalized to unity. If the target point is $O : (\sqrt{2}, 0)$, clearly its distance from the starting point $B : (b\cos\phi, b\sin\phi)$ is $r = \sqrt{(\sqrt{2} - b\cos\phi)^2 + b^2\,\sin^2\phi}$. Thus the original probability $p_4(\mathbf{0})$ is then obtained by averaging $q(\boldsymbol{r})$ over all possible $\phi$ (i.e., all possible $B$'s) with uniform probability

$$p_4(\mathbf{0}) = \frac{1}{2\pi a} \int_0^{2\pi} \delta\left(\sqrt{(\sqrt{2} - b\cos\phi)^2 + b^2\,\sin^2\phi} - a\right) \frac{d\phi}{2\pi}\,. \tag{S6}$$

To perform this integral, we first use the periodicity of the integrand with $\phi$ to rewrite it as

$$p_4(\mathbf{0}) = \frac{1}{2\pi^2\,a} \int_0^{\pi} \delta(\left(\sqrt{(\sqrt{2} - b\cos\phi)^2 + b^2\,\sin^2\phi} - a\right) d\phi\,. \tag{S7}$$

To perform this integral over $\phi$, it is convenient to make a change of variable $\phi \to f(\phi)$ where

$$f(\phi) = \sqrt{(\sqrt{2} - b\cos\phi)^2 + b^2\,\sin^2\phi} - a = \sqrt{b^2 + 2 - 2\sqrt{2}\,b\,\cos(\phi)} - a \tag{S8}$$

and rewrite Eq. (S7) as

$$p_4(\mathbf{0}) = \frac{1}{2\pi^2\,a} \int_0^{\pi} \delta\left(f(\phi)\right) d\phi = \frac{1}{2\pi^2\,a\,|f'(\phi^*)|} \tag{S9}$$

where $f'(\phi) = df(\phi)/d\phi$ and $\phi^* \in [0, \pi]$ is the unique root of $f(\phi^*) = 0$, i.e, upon using Eq. (S8)

$$\cos(\phi^*) = \frac{2 + b^2 - a^2}{2\sqrt{2}\,b}\,. \tag{S10}$$

Evaluating the Jacobian $|f'(\phi^*)|$ and using Eq. (S10) then gives us the desired integral

$$p_4(\mathbf{0}) = \frac{1}{\pi^2}\,\frac{1}{\sqrt{8b^2 - (2b^2 - a^2)^2}}\,. \tag{S11}$$

One can further use the identity, $8b^2 - (2 + b^2 - a^2)^2 = \left((a+b)^2 - 2\right)\left(2 - (a-b)^2\right)$, to re-write the right hand side (rhs) of Eq. (S11) in a way that is manifestly symmetric under the exchange of $a$ and $b$. Thus, the lhs of Eq. (15) of the main text, given by $4\pi^2 p_4(\mathbf{0})$ reduces, using Eq. (S11), to the rhs of Eq. (15) in the main text. This then provides the detailed proof of Eq. (15).

*Proof of Eq. (16).* This proof proceeds in a similar manner as above, except that the jump in the 4-th step (from $B$ on the circle of radius $b$ centered at $O'$ in Fig. S2-b) is no longer a Pearson jump of fixed length $a$ as before, but rather a jump whose endpoint is distributed uniformly *within* a circle of radius $a$ with $a < b$. In other words, the jump pdf of the 4-th step is now $q(\boldsymbol{r}) = \frac{1}{\pi a^2}\theta(a - r)$ where $r = |\boldsymbol{k}r|$ and $\theta(z)$ is the Heaviside step function: $\theta(z) = 1$

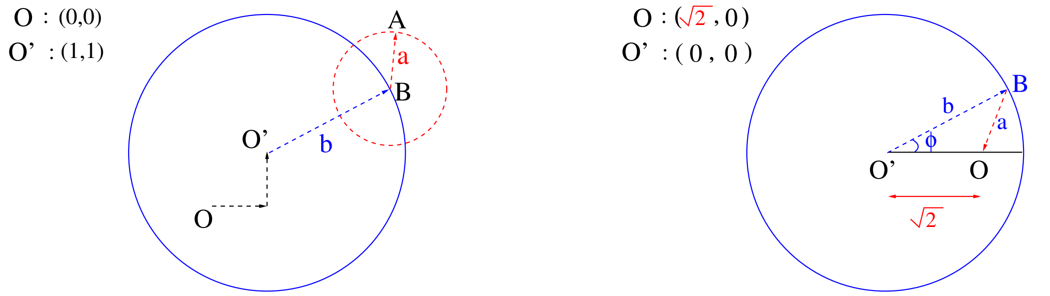


FIG. S2. (a) A random walk, starting at $O:(0,0)$ makes 4 steps: (i) a $+1$ jump along $x$ direction (ii) a $+1$ jump along $y$ direction (iii) a Pearson jump of fixed length $b$, by choosing the point landing point $B$ uniformly on a circle of radius $b$ centered at $O':(1,1)$ and (iv) a Pearson jump of fixed length $a<b$ where the landing point $A$ is chosen uniformly on a circle of radius $a$. (b) To compute the probability (density) $p_4(\mathbf{0})$ of coming back to the origin after 4 steps, it is sufficient to calculate the probability (density) that the walker, starting at point $B$ (chosen uniformly on the circle of radius $b$) after the third step, lands at the point $O:(\sqrt{2},0)$ on the $x$ axis with the new origin $O':(0,0)$.

if $z>0$ and is 0 otherwise. Consider first the lhs of Eq. (16) in the main text. Using line (i) of Eq. (10) with $d=2$ for the 4-th step, we get the probability (density) for the walker to land at the origin

$$p_4(\mathbf{0}) = \frac{1}{2\pi^2 a}\int_{\mathbb{R}^2} dk_x\, dk_y\, \cos(k_x)\, \cos(k_y)\, J_0(b\,k)\, \frac{J_1(a\,k)}{k}\,. \tag{S12}$$

Following the same construction in Fig. S2-b as in the previous case, with the exception that the pdf $q(\boldsymbol{r})$ in the 4-th step is given by $q(\boldsymbol{r})=\frac{1}{\pi a^2}\theta(a-r)$, we get

$$p_4(\mathbf{0}) = \frac{1}{\pi a^2}\int_0^{2\pi} \theta\left(a-\sqrt{(\sqrt{2}-b\cos\phi)^2+b^2\,\sin^2\phi}\right)\frac{d\phi}{2\pi}\,. \tag{S13}$$

We again use the periodicity of the integrand to first re-write this as

$$p_4(\mathbf{0}) = \frac{1}{\pi^2 a^2}\int_0^{\pi} \theta\left(a-\sqrt{(\sqrt{2}-b\cos\phi)^2+b^2\,\sin^2\phi}\right) d\phi\,. \tag{S14}$$

However the integral on the rhs can now be trivially done to give

$$p_4(\mathbf{0}) = \frac{1}{\pi^2 a^2}\,\phi^* \tag{S15}$$

where again $\phi^*$ is given by the root $f(\phi^*)=0$, i.e., by Eq. (S10). Using this we get

$$p_4(\mathbf{0}) = \frac{1}{\pi^2 a^2}\,\arccos\left(\frac{2+b^2-a^2}{2\sqrt{2}\,b}\right)\,. \tag{S16}$$

Comparing to Eq. (S12) then provides a proof of Eq. (16) in the main text.

## III. ANOTHER FAMILY OF RELATIONS INVOLVING A MOMENT OF THE WALKERS PROBABILITY DISTRIBUTION

In the main text, we solved non trivial integrals by establishing a mapping to the density of random walkers at some point in space, when the underlying walk is made of finite-range jumps. A related approach takes advantage of a specific feature of such walks. We consider a random walk on the line, with a Pearson first jump: the walker is then at $x=\pm a_1$ and $\langle |x_1|\rangle = a_1$ after step 1. If the following steps are left-right symmetric, bounded with amplitude $a_n$ ($n=2,3...N$) such that the walkers cannot go back to the origin after $N$ steps, then $\langle |x_N|\rangle = a_1$ also; this is the case provided $\sum_{n=2}^{N} a_n < a_1$, which we henceforth assume. Indeed, if the walker is at $x=a_1$ after step 1, then its mean position remains at $a_1$ for all successive steps. Since the walker cannot reach the origin after $N$ steps, its position

remain positive, so that $x_N$ and $|x_N|$ have the same mean value. Clearly, a related argument holds when the walker is at $-a_1$ after step 1, from which we have $\langle |x_1| \rangle = a_1$.

The remaining task is to relate $\langle |x_N| \rangle$ to the characteristic function of the $N$-step random walk. The following identity is thus of particular interest:

$$|y| \;=\; \frac{2}{\pi}\int_0^\infty \frac{1-\cos(ky)}{k^2}\,dk, \tag{S17}$$

which holds for all real $y$. Choosing $y = x_N$ and taking the mean value of this relation, we get

$$\langle |x_N| \rangle \;=\; \frac{2}{\pi}\int_0^\infty \frac{1-\langle\, \exp(i\,k\,x_N)\,\rangle}{k^2}\,dk \tag{S18}$$

where we have used the fact that the imaginary part of the integral vanishes. Next, using the explicit expression for the characteristic function $\langle \exp(i\,k\,x_N)\rangle$ (where the first jump is Pearson's type with fixed length $a_1$ and successive jumps have independent but arbitrary distributions but each with a finite support), we obtain the relation

$$\int_0^\infty \frac{1}{k^2}\left(1-\cos\left(ka_1\right)\prod_{n=2}^{N}\widehat{\mathcal{F}}_n(a_n k)\right)dk \;=\; \frac{\pi}{2}\,a_1, \qquad \text{provided} \quad \sum_{n=2}^{N} a_n < a_1, \tag{S19}$$

where each "building block" $\widehat{\mathcal{F}}_n$ has the same meaning as in the main text (Fourier transform of an arbitrary distribution with unit-support). In particular, we may choose the first $N_1$ jumps to be of Pearson's type and the next $N_2$ terms of uniform jump distribution and obtain the nontrivial identity

$$\int_0^\infty \frac{1-\prod_{n=1}^{N_1}\cos(a_n k)\prod_{n'=1}^{N_2}\mathrm{sinc}(b_{n'}k)}{k^2}\,dk \;=\; \frac{\pi}{2}\,a_1, \qquad \text{provided} \quad \sum_{n=2}^{N_1} a_n + \sum_{n'=1}^{N_2} b_{n'} < a_1, \tag{S20}$$

taking again, without loss of generality, positive $a_n$ and $b_{n'}$. For concreteness, we plot in Fig. S3 the probability density of a 4-step walk corresponding to the relation

$$\frac{2}{\pi}\int_0^\infty \frac{1-\cos(k)\,\cos(k/2)\,\mathrm{sinc}(k/4)\,\mathrm{sinc}(k/8)}{k^2}\,dk \;=\; 1. \tag{S21}$$

These results, unfortunately, cannot be easily generalized to arbitrary dimensions $d > 1$.

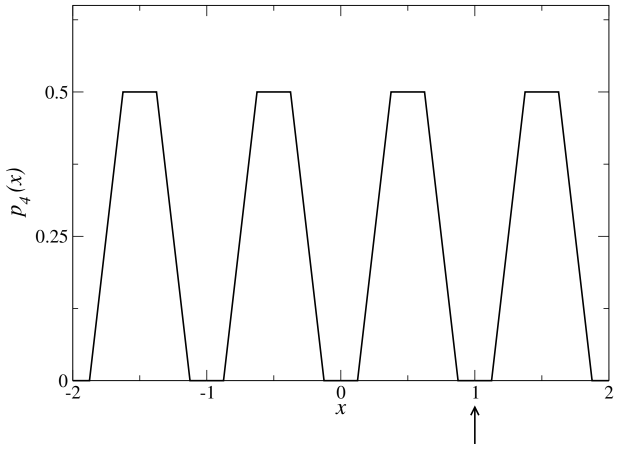


FIG. S3. Probability density function with $N = 4$: the first two steps are Pearson-type with amplitude 1 and 1/2, and the last two steps are uniform in $[-1/4, 1/4]$ and $[-1/8, 1/8]$. Symmetry implies that $\langle |x_4| \rangle = 1$, which in turn leads to relation (S21). Here, it can be considered that the message starts at $|x| = 1$ after the first step (see the arrow), and travels towards the origin at $x = 0$ that can be viewed as a boundary. Since the space covered by the sum of the second, third and fourth steps is bounded by $1/2 + 1/4 + 1/8 < 1$, the origin is void of walkers and symmetry applies ($\langle |x_4| \rangle = 1$).

## IV. DO THE $\widehat{\mathcal{F}}_n^{(d)}(\boldsymbol{k})$ NEED TO BE CHARACTERISTIC FUNCTIONS?

The answer is negative, and follows from a two-pronged argument. First, one can use the Plancherel theorem to write integrals like those of (11) or (13) as integrals over $\boldsymbol{x}$ rather than $\boldsymbol{k}$. For concreteness, we consider (11), and for simplicity, we work out the case $d = 1$, making use of (10)

$$\int_{\mathbb{R}} \mathrm{sinc}(a_1 k) \prod_{n=2}^{N} \widehat{\mathcal{F}}_n(a_n\, k)\, \frac{dk}{2\pi} = \int_{\mathbb{R}} \frac{\theta(1-|x|)}{2a_1} \circledast_{n=2}^{N} \mathcal{F}_n(a_n\, x)\, dx, \tag{S22}$$

where $\theta$ denotes Heaviside step function, and the $\mathcal{F}_n(x)$ are of support bounded by unity. Since the convolution product $\circledast_{n=2}^{N} \mathcal{F}_n(a_n\, x)$ yields a bounded function of support smaller than $\sum_{n=2}^{N} a_n$, assumed to be smaller than $a_1$, we have

$$\int_{\mathbb{R}} \theta(1-|x|) \circledast_{n=2}^{N} \mathcal{F}_n(a_n\, x)\, dx = \int_{\mathbb{R}} \circledast_{n=2}^{N} \mathcal{F}_n(a_n\, x)\, dx. \tag{S23}$$

The integral on the rhs can be viewed as the Fourier Transform of the convolution, evaluated at $k = 0$. This means finally that

$$\int_{\mathbb{R}} \mathrm{sinc}(a_1 k) \prod_{n=2}^{N} \widehat{\mathcal{F}}_n(a_n\, \boldsymbol{k})\, \frac{dk}{2\pi} = \frac{1}{2a_1} \prod_{n=2}^{N} \widehat{\mathcal{F}}_n(0), \tag{S24}$$

which can be rewritten

$$\int_{\mathbb{R}} \frac{J_{1/2}(a_1 k)}{k^{1/2}} \prod_{n=2}^{N} \widehat{\mathcal{F}}_n(a_n\, k)\, dk = \left(\frac{2\pi}{a_1}\right)^{1/2} \prod_{n=2}^{N} \widehat{\mathcal{F}}_n(0). \tag{S25}$$

In the most general $d$-dimensional case where the $\widehat{\mathcal{F}}_n^{(d)}(\boldsymbol{k})$ are not characteristic functions but only of bounded Fourier transform, (13) remains true while (11) becomes

$$\int_{\mathbb{R}^d} \frac{J_{d/2}(a_1 k)}{k^{d/2}} \prod_{n=2}^{N} \widehat{\mathcal{F}}_n^{(d)}(a_n\, \boldsymbol{k})\, d^d\boldsymbol{k} = \left(\frac{2\pi}{a_1}\right)^{d/2} \prod_{n=2}^{N} \widehat{\mathcal{F}}_n^{(d)}(\boldsymbol{0}) \tag{S26}$$

once more under the proviso that $\sum_{n=2}^{N} a_n < a_1$.

---

[1] D. Borwein and J. Borwein, The Ramanujan Journal **5**, 73 (2001); D. Borwein, J.M. Borwein and A. Straub, American Mathematical Monthly **119**, 535 (2012).
[2] H. Schmid, Elem. Math. **69**, 11 (2014).
